# Supplementary material for: Novel digital tissue phenotypic signatures of distant metastasis in colorectal cancer
Source: arXiv:1801.07451 source file (2018-01-23)
Supplement: Supplementary file 1 [file Supplementary_Materials.pdf]

# Supplementary Information:
# Novel Digital Tissue Phenotypic Signatures of Distant Metastasis in Colorectal Cancer

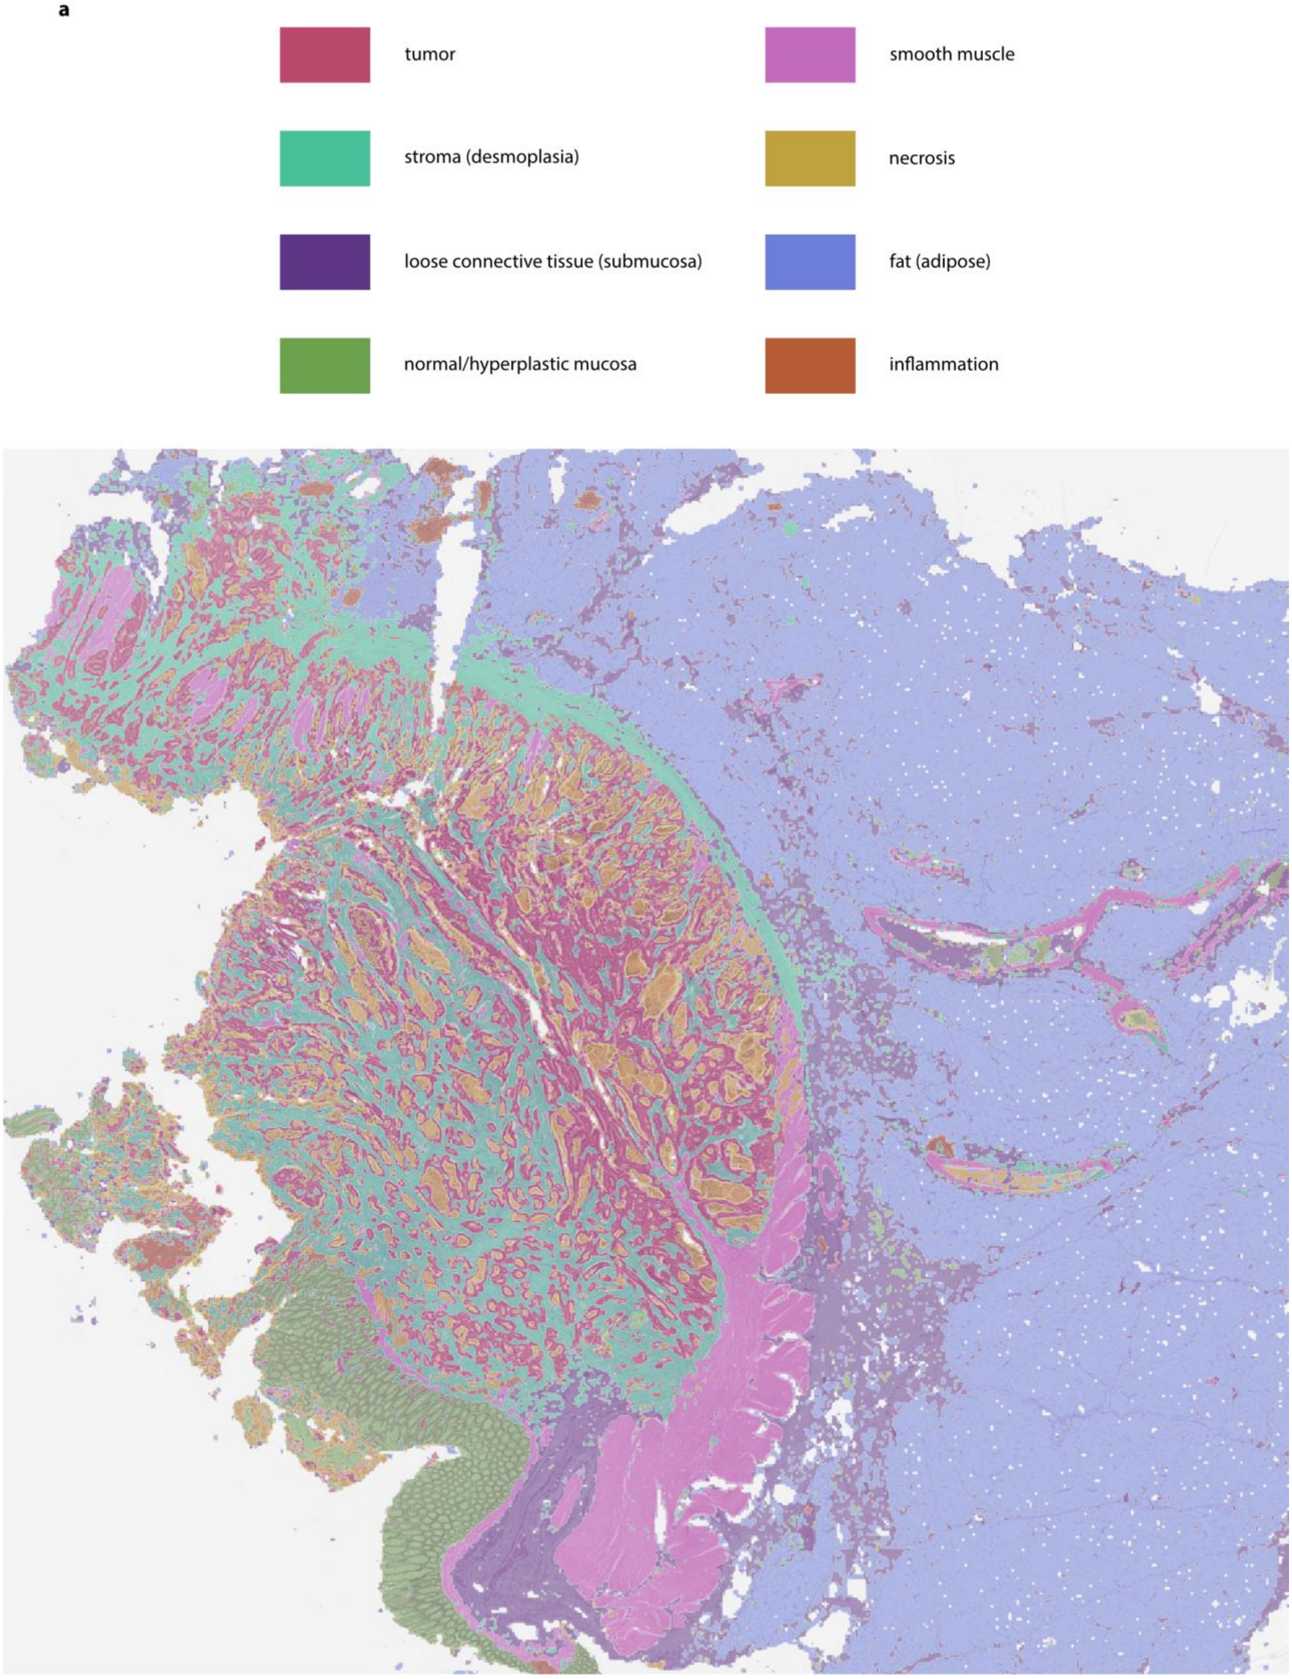

b

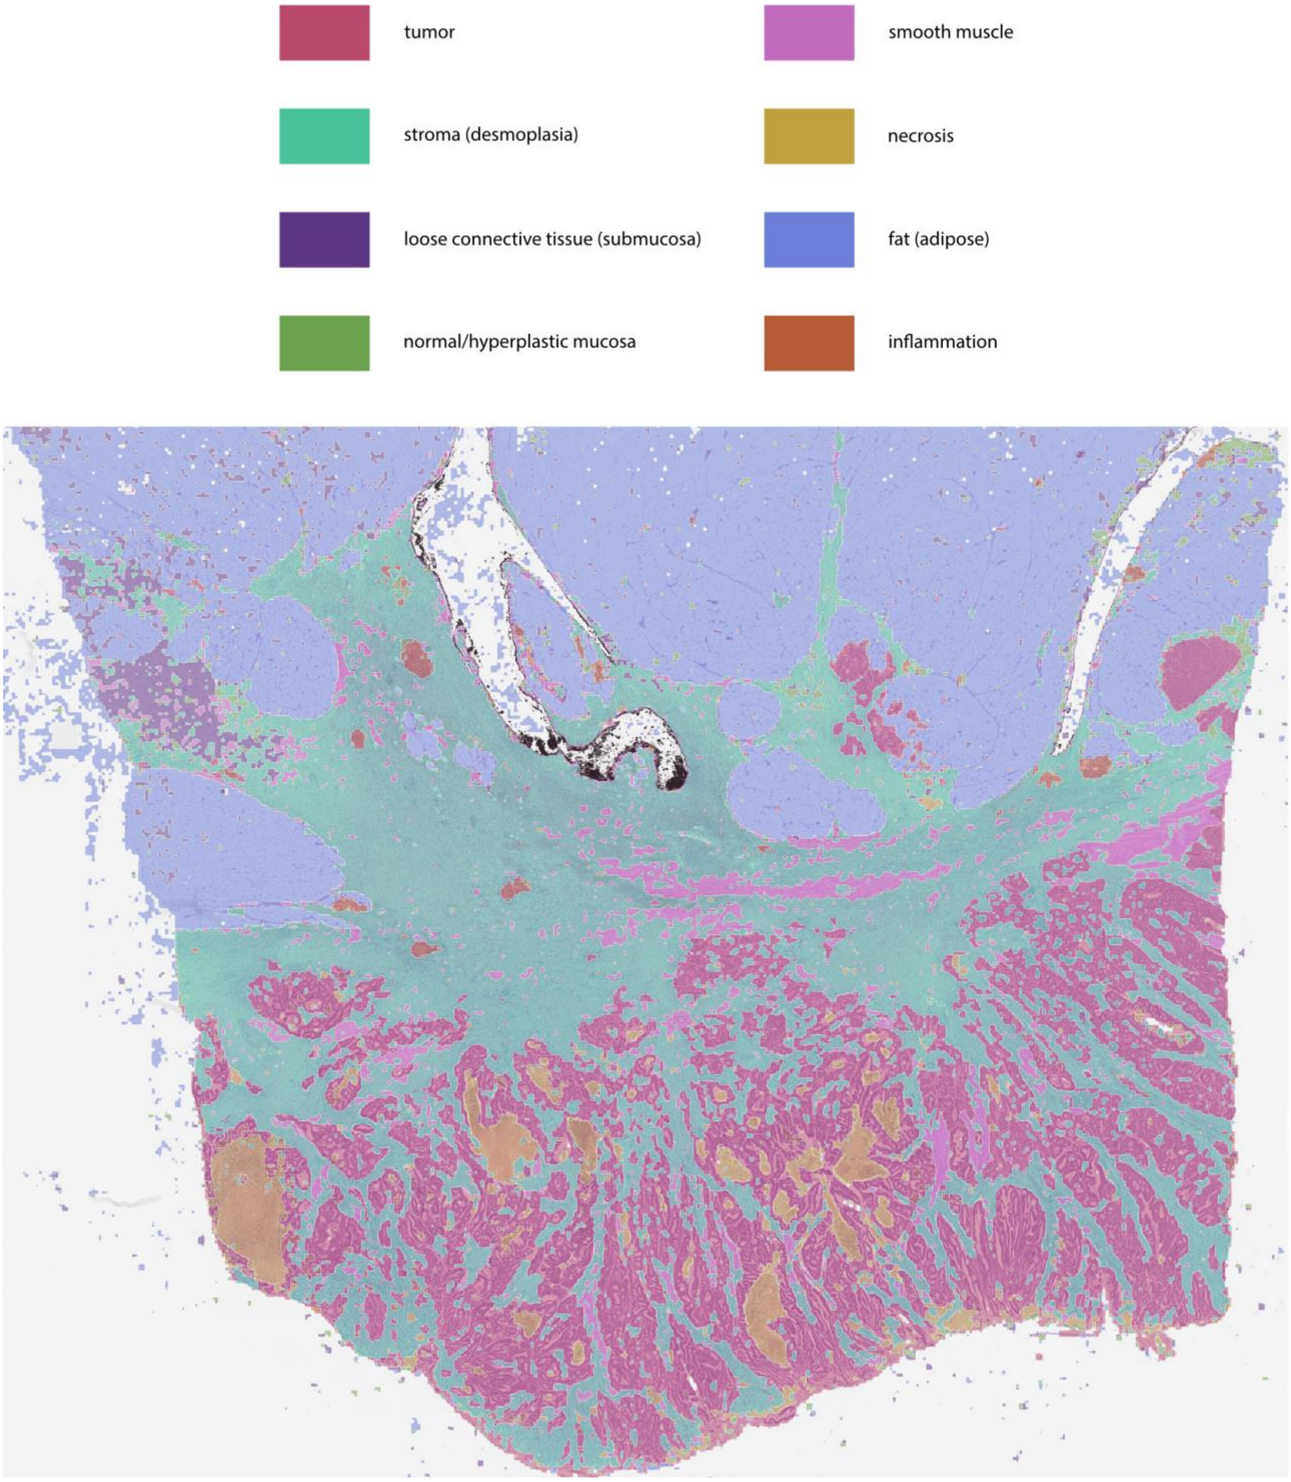
tumor
smooth muscle
stroma (desmoplasia)
necrosis
loose connective tissue (submucosa)
fat (adipose)
normal/hyperplastic mucosa
inflammation

c

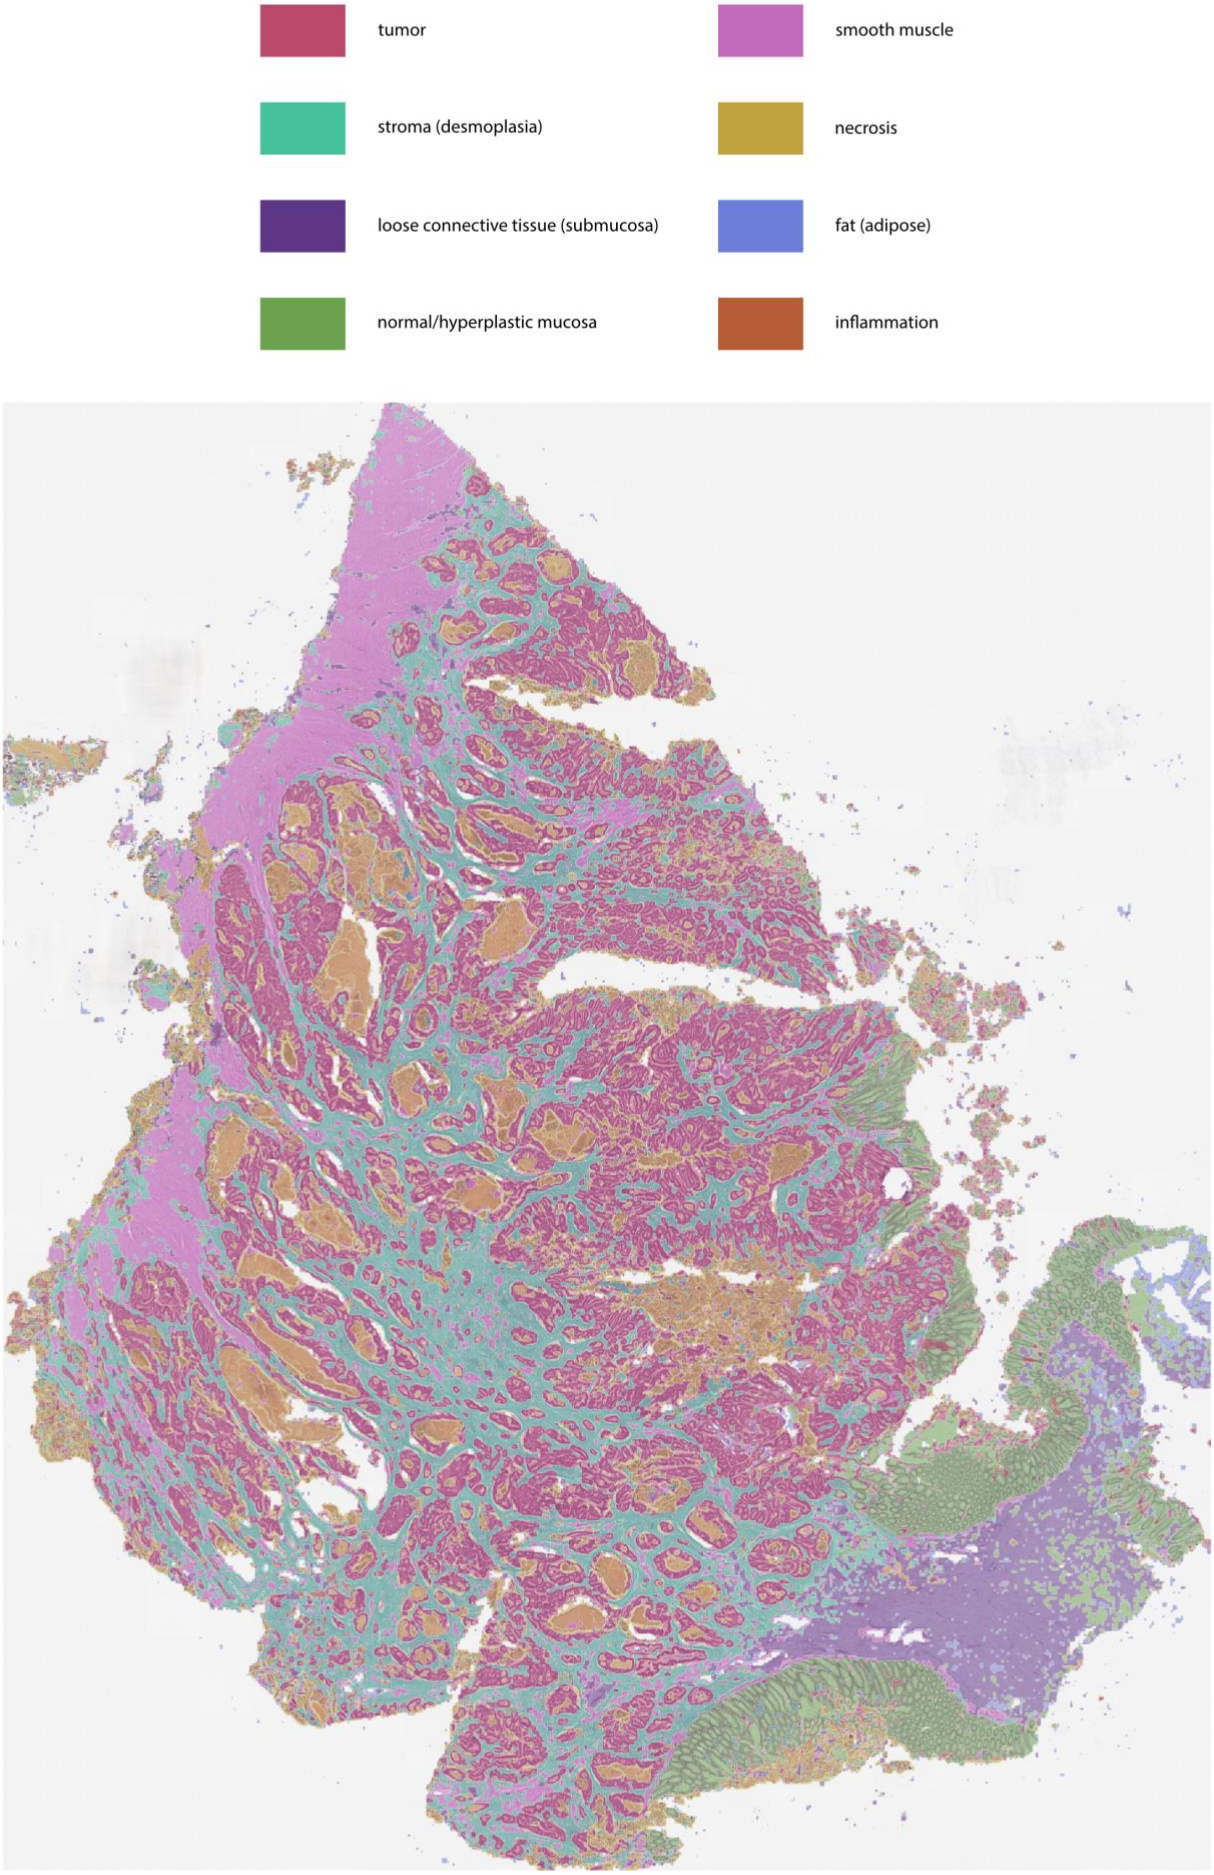
tumor
smooth muscle
stroma (desmoplasia)
necrosis
loose connective tissue (submucosa)
fat (adipose)
normal/hyperplastic mucosa
inflammation

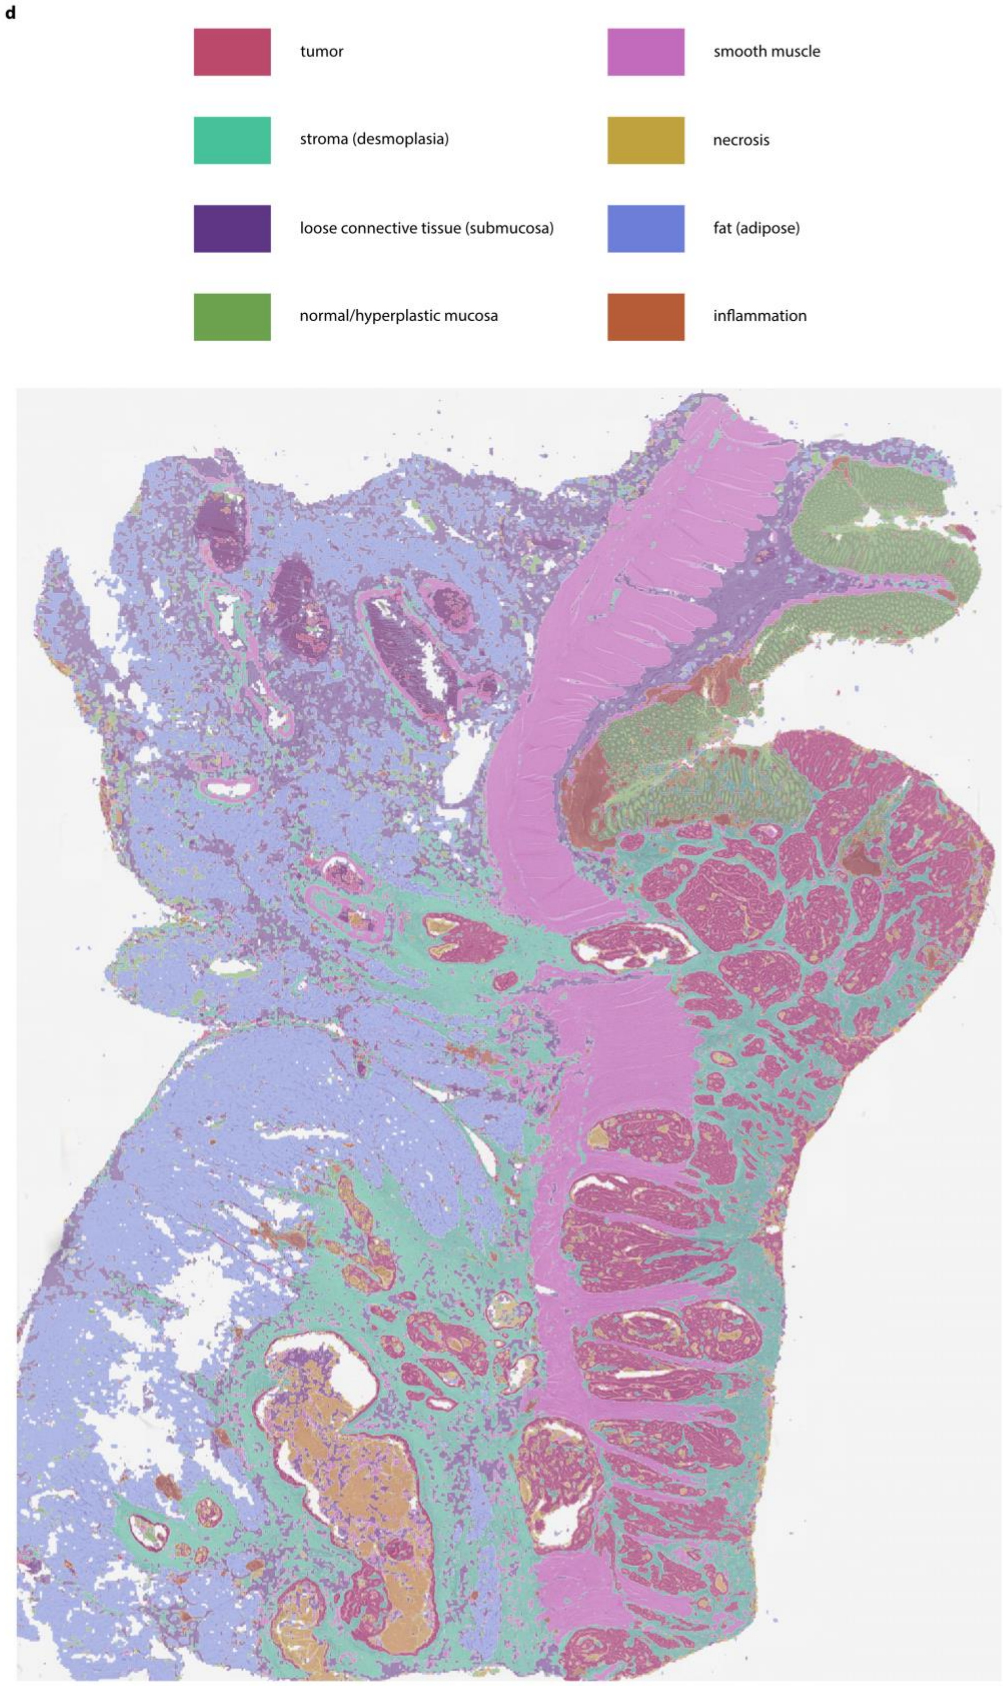


**Fig. S1.** Example of segmentation results.

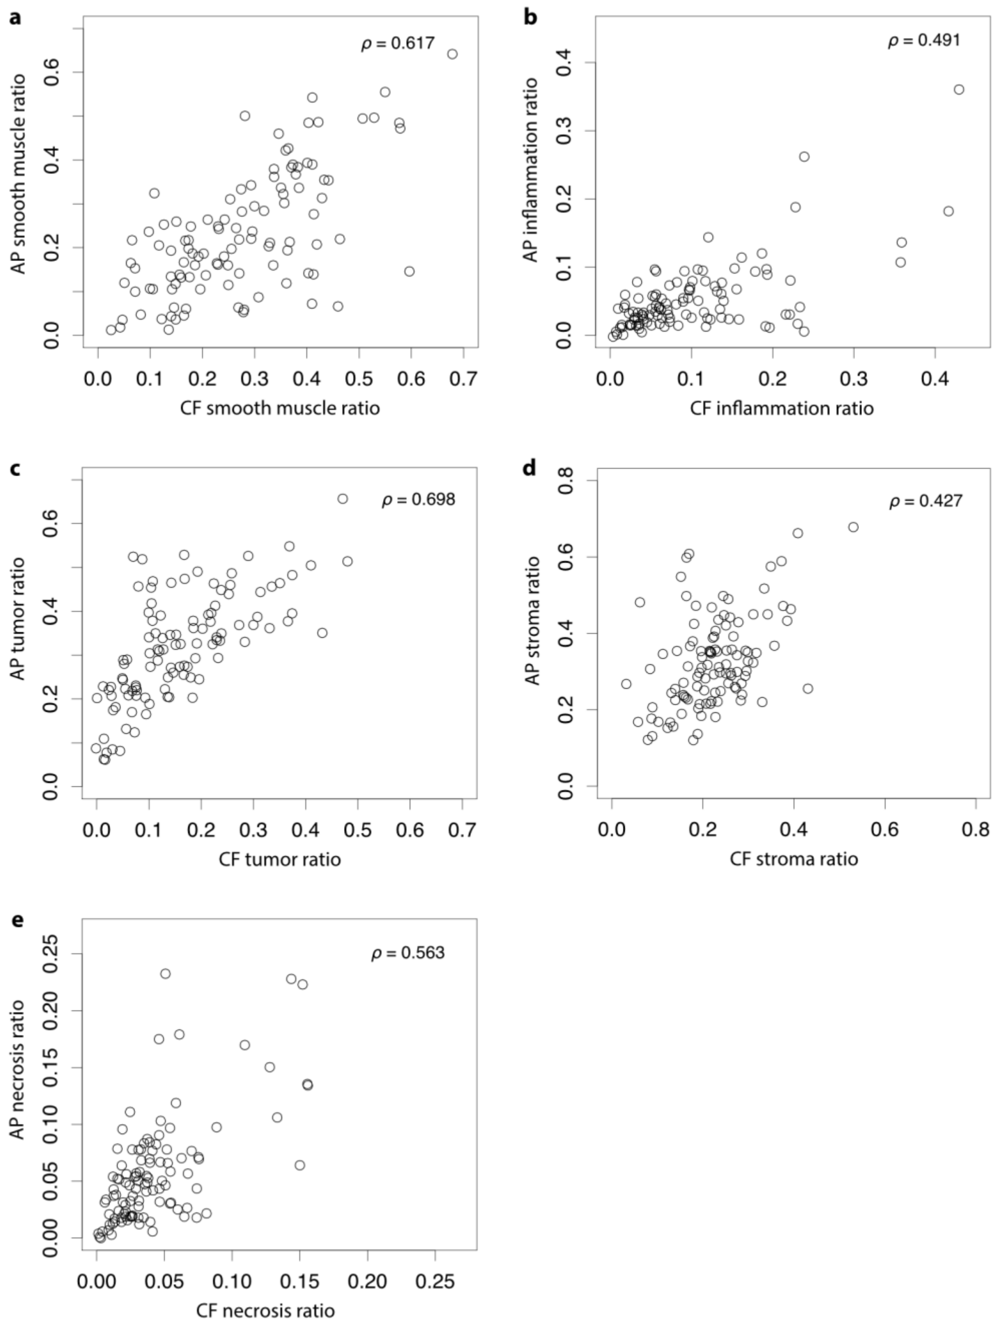


**Fig. S2.** Correlation between the corresponding CF and AP tissue phenotypic features. The correlation is measured by Spearman correlation coefficient $\rho$.

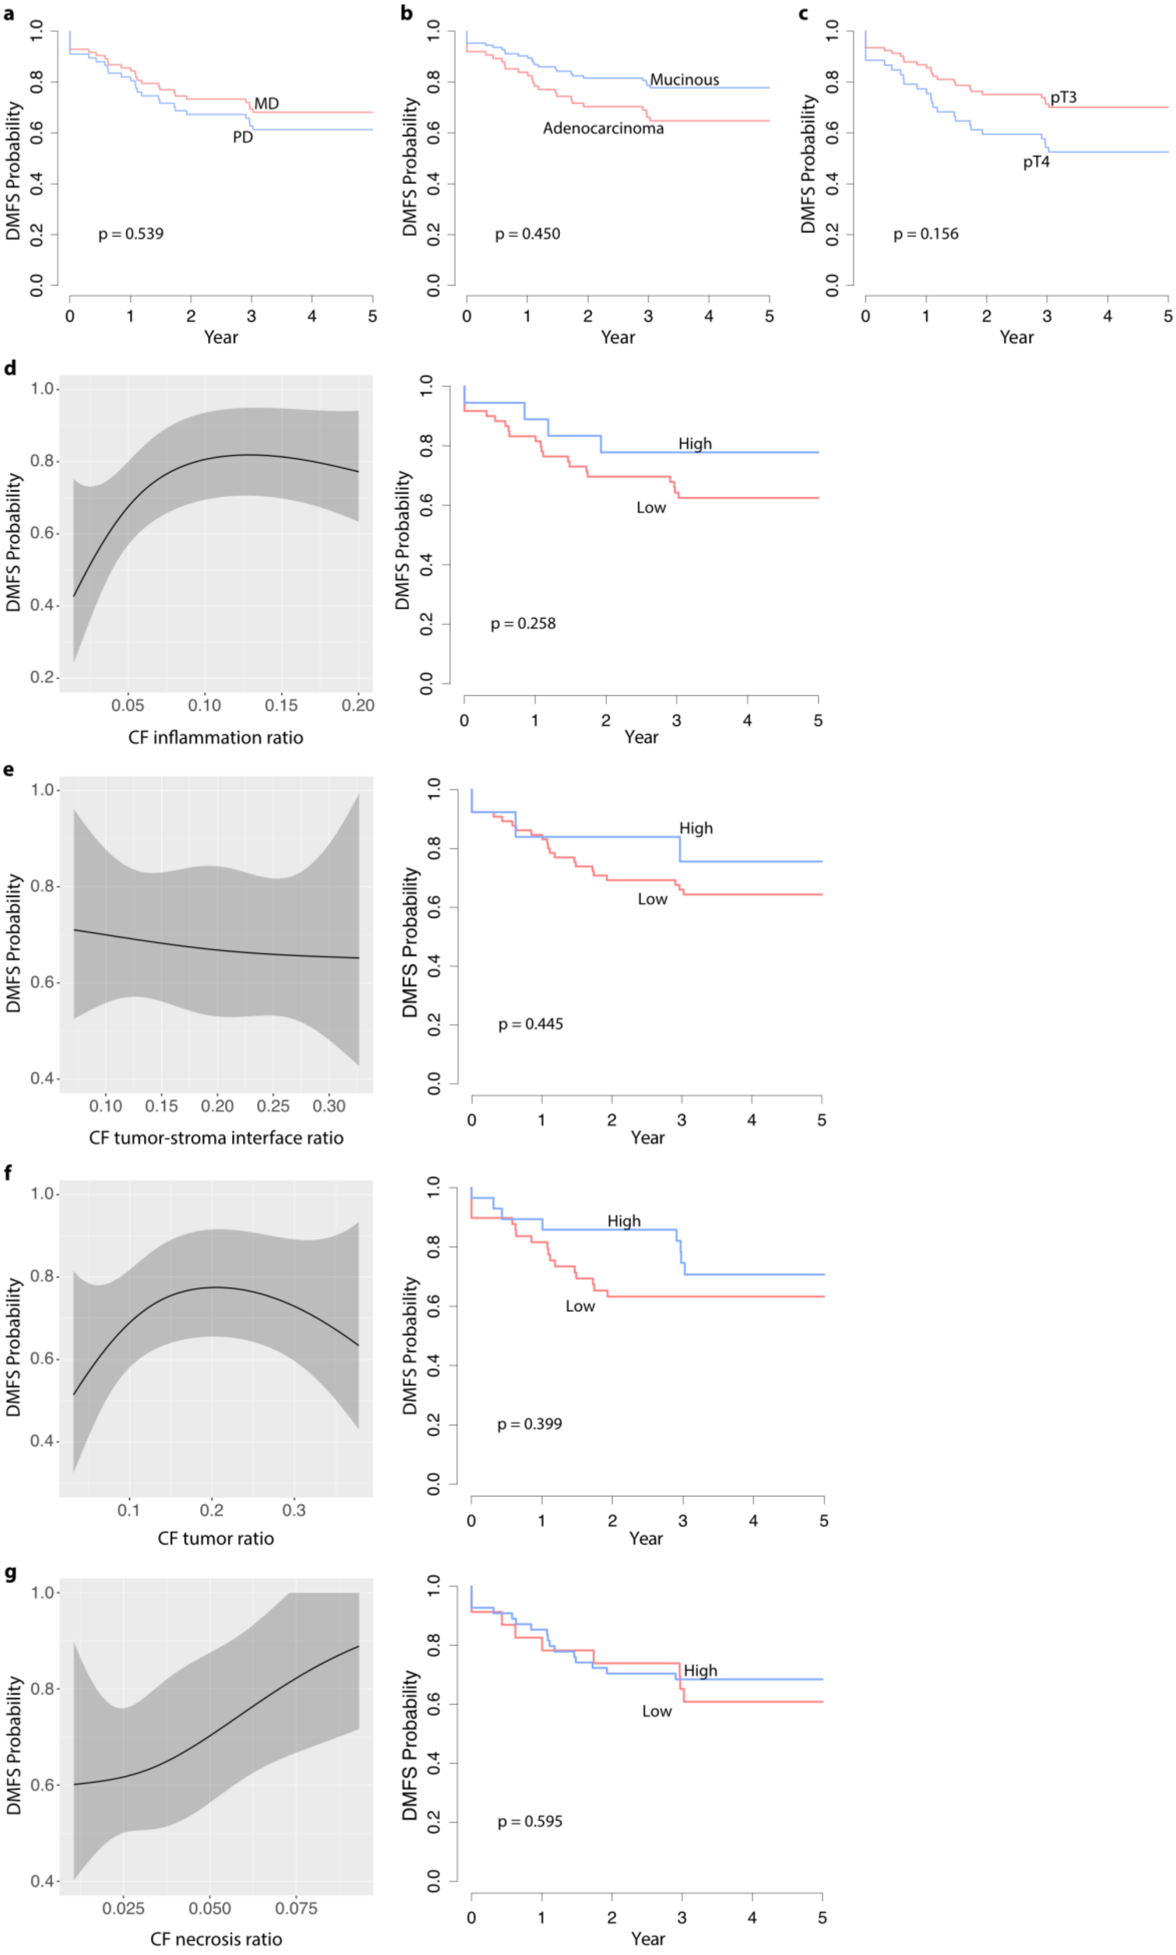
a
DMFS Probability
Year
MD
PD
p = 0.539
b
DMFS Probability
Year
Mucinous
Adenocarcinoma
p = 0.450
c
DMFS Probability
Year
pT3
pT4
p = 0.156
d
DMFS Probability
CF inflammation ratio
DMFS Probability
Year
High
Low
p = 0.258
e
DMFS Probability
CF tumor-stroma interface ratio
DMFS Probability
Year
High
Low
p = 0.445
f
DMFS Probability
CF tumor ratio
DMFS Probability
Year
High
Low
p = 0.399
g
DMFS Probability
CF necrosis ratio
DMFS Probability
Year
High
Low
p = 0.595

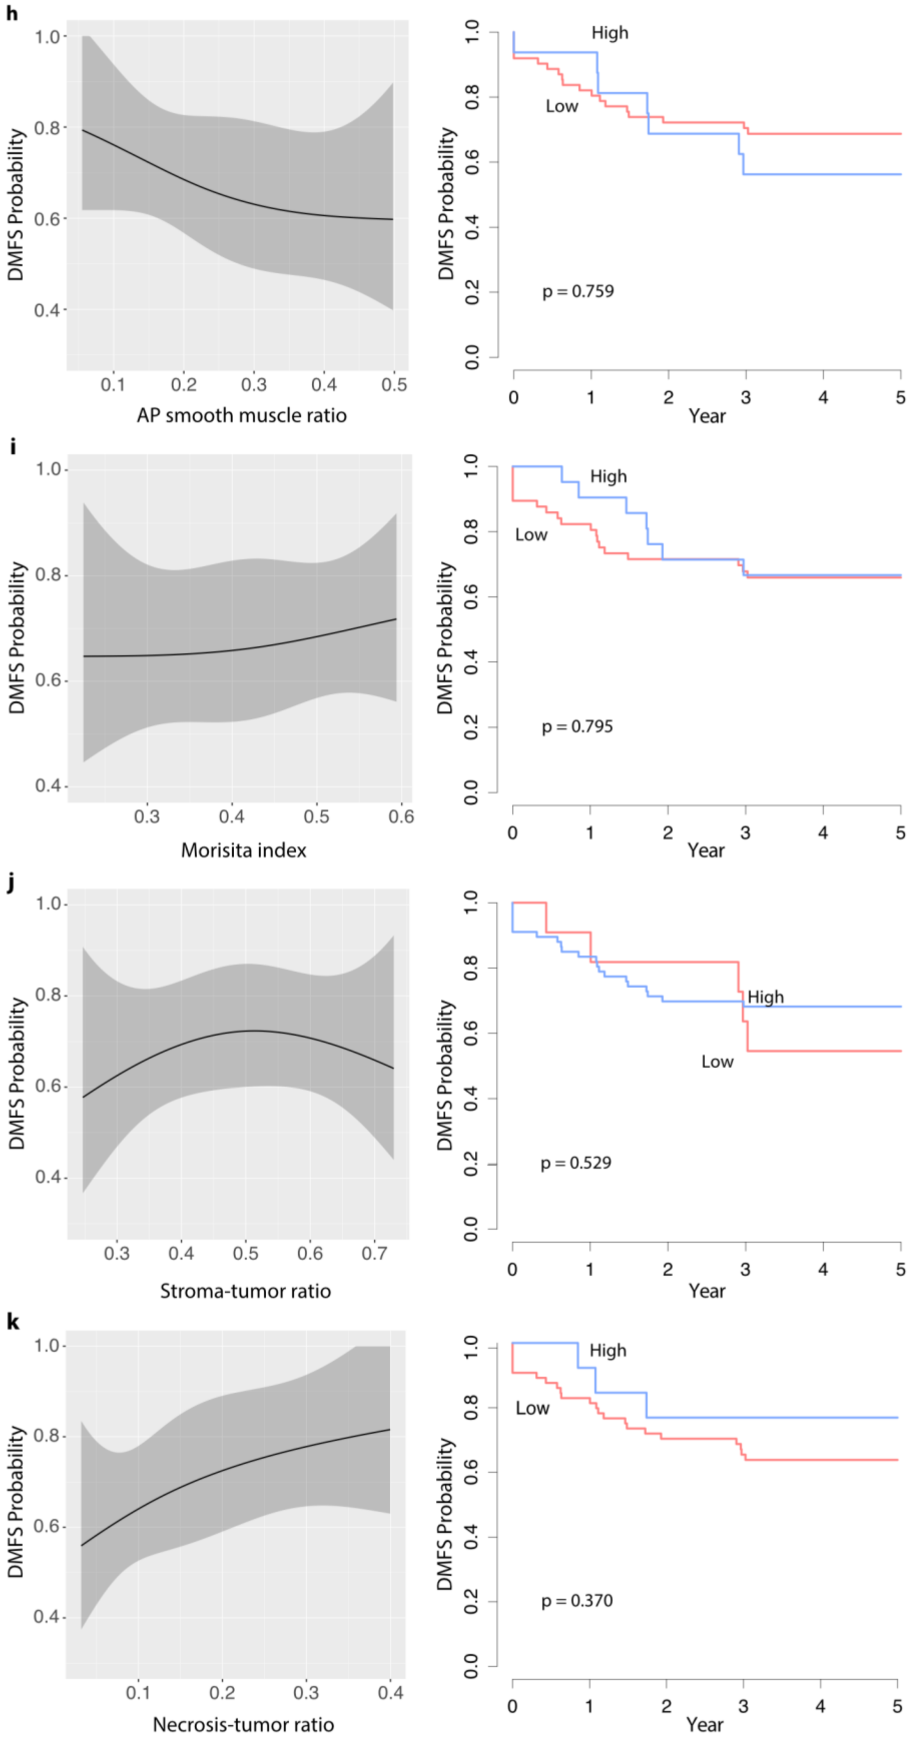
h
DMFS Probability
AP smooth muscle ratio
High
Low
p = 0.759
Year
i
DMFS Probability
Morisita index
High
Low
p = 0.795
Year
j
DMFS Probability
Stroma-tumor ratio
High
Low
p = 0.529
Year
k
DMFS Probability
Necrosis-tumor ratio
High
Low
p = 0.370
Year

**Fig. S3.** Univariate survival analysis on the UHCW cohort. Kaplan-Meier curves stratified by tumor differentiation (**a**), tumor histological type (**b**), primary tumor (T) stage (**c**), CF inflammation ratio (**d**, *right*), CF tumor-stroma interface ratio (**e**, *right*), CF tumor ratio (**f**, *right*), CF necrosis ratio (**g**, *right*), AP smooth muscle ratio, (**h**, *right*) Morisita index (**i**, *right*), stroma-tumor ratio (**j**, *right*), and necrosis-tumor ratio (**k**, *right*). The log-rank p-value is calculated for each variable to assess if there exists a statistically significant difference between the survival distributions of different strata within the variable. The 5-year survival estimates with respect to CF inflammation ratio (**d**, *left*) CF tumor-stroma interface ratio (**e**, *left*), CF tumor ratio (**f**, *left*), CF necrosis ratio (**g**, *left*), AP smooth muscle ratio (**h**, *left*), Morisita index (**i**, *left*), and stroma-tumor ratio (**j**, *left*), and necrosis-tumor ratio (**k**, *right*). The shaded gray areas correspond to the 95% confidence intervals of the estimates.

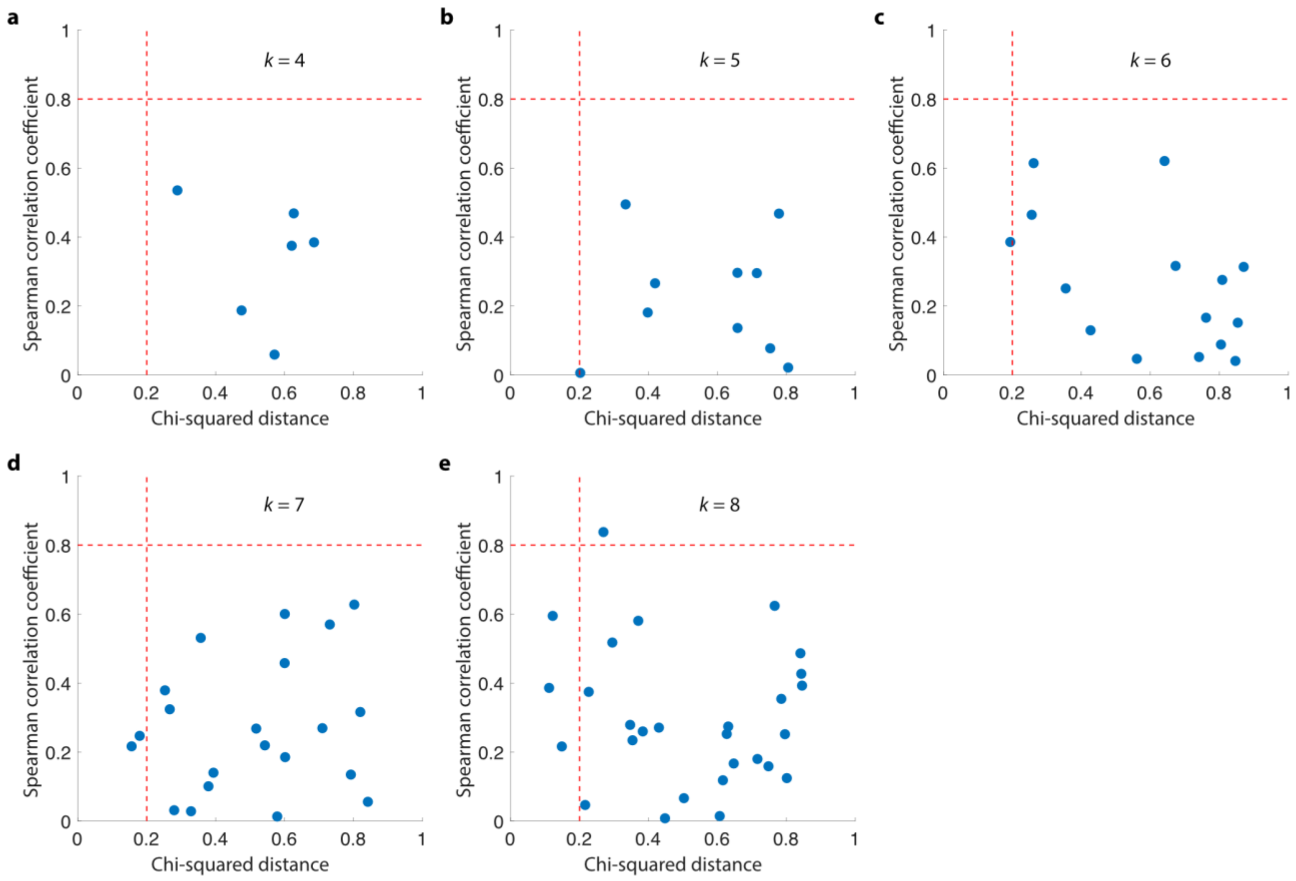


**Fig. S4**. Selection of the number of cell-cell connection frequency based tissue phenotypes. In determining the number of phenotypes (*k*), two criteria are taken into account: 1) similarity between phenotypes, and 2) correlation between features calculated based on the phenotypes. Each tissue phenotype should be less similar to the others and the features derived from these phenotypes should be less correlated. We measure the similarity between a pair of phenotypes in terms of a chi-squared distance between medoids that represent them. Then we calculate a feature value for each individual phenotype as the ratio of the area of that tissue phenotype to the total tissue area, and we compute the correlation between a pair of features using Spearman correlation coefficient. The chi-squared distance which is less than 0.2 (vertical red line) and the Spearman correlation coefficient which is greater than 0.8 (horizontal red line) are considered undesirable. The figures show the relationship between the chi-squared distance and the Spearman correlation coefficient of individual pairs of phenotypes with respect to *k* = 4 (**a**), *k* = 5 (**b**), *k* = 6 (**c**), *k* = 7 (**d**), and *k* = 8 (**e**). We select the number of phenotypes as *k* = 6 since it is the largest number that still retains the desirable distance and correlation for all pairs of phenotypes.

**Table S1.** Prognostic values of different features according to multivariate logistic regression analysis.

| Feature | Feature value | | Odds ratio factor | | | Likelihood ratio test p-value | AUC |
|---|---|---|---|---|---|---|---|
| | Baseline | Change | Estimate | Lower 95% CI | Upper 95% CI | | |
| Connection frequency based tissue phenotypic features | | | | | | | |
| **CF smooth muscle ratio** | 0.167 | 0.372 | 2.350 | 1.132 | 4.876 | **0.008*** | 0.623 |
| Differentiation | MD | PD | 1.382 | 0.451 | 4.23 | 0.708 | |
| Histological type | Adenocarcinoma | Mucinous | 0.591 | 0.134 | 2.603 | 0.426 | |
| T stage | pT3 | pT4 | 2.673 | 0.935 | 7.640 | 0.054 | |
| **CF inflammation ratio** | 0.042 | 0.138 | 0.307 | 0.126 | 0.749 | **0.022*** | 0.582 |
| Differentiation | MD | PD | 1.129 | 0.373 | 3.414 | 0.872 | |
| Histological type | Adenocarcinoma | Mucinous | 0.68 | 0.162 | 2.859 | 0.544 | |
| T stage | pT3 | pT4 | 1.989 | 0.703 | 5.625 | 0.185 | |
| **CF tumor-stroma interface ratio** | 0.122 | 0.229 | 1.177 | 0.623 | 2.224 | 0.800 | 0.530 |
| Differentiation | MD | PD | 1.577 | 0.558 | 4.460 | 0.415 | |
| Histological type | Adenocarcinoma | Mucinous | 0.624 | 0.149 | 2.612 | 0.480 | |
| T stage | pT3 | pT4 | 2.216 | 0.757 | 6.486 | 0.124 | |
| **CF tumor ratio** | 0.079 | 0.229 | 0.52 | 0.252 | 1.070 | 0.187 | 0.566 |
| Differentiation | MD | PD | 1.348 | 0.448 | 4.052 | 0.626 | |
| Histological type | Adenocarcinoma | Mucinous | 0.683 | 0.163 | 2.867 | 0.564 | |
| T stage | pT3 | pT4 | 2.11 | 0.763 | 5.836 | 0.135 | |
| **CF stroma ratio** | 0.174 | 0.275 | 0.585 | 0.34 | 1.007 | 0.139 | 0.616 |
| Differentiation | MD | PD | 1.564 | 0.541 | 4.521 | 0.442 | |
| Histological type | Adenocarcinoma | Mucinous | 0.682 | 0.162 | 2.865 | 0.549 | |
| T stage | pT3 | pT4 | 2.114 | 0.76 | 5.880 | 0.133 | |
| **CF necrosis ratio** | 0.022 | 0.053 | 0.738 | 0.371 | 1.469 | 0.254 | 0.552 |
| Differentiation | MD | PD | 1.942 | 0.644 | 5.859 | 0.288 | |
| Histological type | Adenocarcinoma | Mucinous | 0.692 | 0.165 | 2.894 | 0.568 | |
| T stage | pT3 | pT4 | 2.125 | 0.769 | 5.868 | 0.116 | |
| **CF smooth muscle ratio** | 0.167 | 0.372 | 2.496 | 0.907 | 6.872 | 0.080 | 0.637 |
| **CF inflammation ratio** | 0.042 | 0.138 | 0.649 | 0.209 | 2.014 | 0.231 | |
| Differentiation | MD | PD | 1.127 | 0.349 | 3.634 | 0.956 | |
| Histological type | Adenocarcinoma | Mucinous | 0.582 | 0.131 | 2.593 | 0.414 | |
| T stage | pT3 | pT4 | 2.723 | 0.895 | 8.283 | 0.070 | |
| Appearance based tissue phenotypic features | | | | | | | |
| **AP smooth muscle ratio** | 0.136 | 0.33 | 2.075 | 0.97 | 4.437 | 0.125 | 0.563 |
| Differentiation | MD | PD | 1.799 | 0.606 | 5.346 | 0.254 | |
| Histological type | Adenocarcinoma | Mucinous | 0.496 | 0.113 | 2.166 | 0.301 | |
| T stage | pT3 | pT4 | 3.225 | 1.062 | 9.788 | **0.028*** | |
| **AP inflammation ratio** | 0.025 | 0.07 | 0.472 | 0.225 | 0.987 | 0.056 | 0.625 |
| Differentiation | MD | PD | 1.387 | 0.475 | 4.057 | 0.558 | |
| Histological type | Adenocarcinoma | Mucinous | 0.738 | 0.170 | 3.197 | 0.650 | |
| T stage | pT3 | pT4 | 2.008 | 0.708 | 5.694 | 0.174 | |
| Other features | | | | | | | |
| **Morisita index (*Maley*)** | 0.344 | 0.529 | 0.868 | 0.461 | 1.632 | 0.866 | 0.502 |
| Differentiation | MD | PD | 1.599 | 0.553 | 4.626 | 0.409 | |
| Histological type | Adenocarcinoma | Mucinous | 0.685 | 0.164 | 2.867 | 0.568 | |
| T stage | pT3 | pT4 | 2.309 | 0.84 | 6.347 | 0.091 | |
| **Stroma-tumor ratio (*Mesker, West, Huijbers*)** | 0.400 | 0.613 | 0.852 | 0.481 | 1.509 | 0.329 | 0.515 |
| Differentiation | MD | PD | 1.475 | 0.505 | 4.309 | 0.472 | |
| Histological type | Adenocarcinoma | Mucinous | 0.807 | 0.189 | 3.443 | 0.749 | |
| T stage | pT3 | pT4 | 2.288 | 0.837 | 6.255 | 0.094 | |
| **Necrosis-tumor ratio (*Pollheimer, Richards, Jayasinghe*)** | 0.077 | 0.224 | 0.577 | 0.278 | 1.197 | 0.272 | 0.575 |
| Differentiation | MD | PD | 1.763 | 0.589 | 5.283 | 0.346 | |
| Histological type | Adenocarcinoma | Mucinous | 0.621 | 0.147 | 2.616 | 0.482 | |
| T stage | pT3 | pT4 | 2.056 | 0.743 | 5.686 | 0.137 | |

* statistically significant result at the 0.05 significance level

**Table S2.** Prognostic values of different features according to the multivariate Cox proportional hazards regression analysis on the UHCW cohort.

| Feature | Feature value | | Hazard ratio factor | | | Wald test p-value | AUC |
|---|---|---|---|---|---|---|---|
| | Baseline | Change | Estimate | Lower 95% CI | Upper 95% CI | | |
| Connection frequency based tissue phenotypic features | | | | | | | |
| **CF smooth muscle ratio** | 0.188 | 0.388 | 2.467 | 1.062 | 5.73 | **0.008*** | 0.623 |
| Differentiation | MD | PD | 1.011 | 0.394 | 2.595 | 0.982 | |
| Histological type | Adenocarcinoma | Mucinous | 0.473 | 0.11 | 2.039 | 0.315 | |
| T stage | pT3 | pT4 | 2.568 | 1.045 | 6.311 | **0.04*** | |
| **CF inflammation ratio** | 0.037 | 0.102 | 0.413 | 0.201 | 0.849 | 0.051 | 0.582 |
| Differentiation | MD | PD | 0.941 | 0.361 | 2.449 | 0.9 | |
| Histological type | Adenocarcinoma | Mucinous | 0.535 | 0.125 | 2.289 | 0.399 | |
| T stage | pT3 | pT4 | 1.816 | 0.775 | 4.258 | 0.17 | |
| **CF tumor-stroma interface ratio** | 0.124 | 0.238 | 1.054 | 0.575 | 1.934 | 0.968 | 0.53 |
| Differentiation | MD | PD | 1.164 | 0.452 | 3.003 | 0.753 | |
| Histological type | Adenocarcinoma | Mucinous | 0.547 | 0.127 | 2.348 | 0.417 | |
| T stage | pT3 | pT4 | 1.801 | 0.751 | 4.319 | 0.187 | |
| **CF tumor ratio** | 0.079 | 0.221 | 0.601 | 0.304 | 1.184 | 0.276 | 0.566 |
| Differentiation | MD | PD | 1.163 | 0.434 | 3.116 | 0.763 | |
| Histological type | Adenocarcinoma | Mucinous | 0.601 | 0.139 | 2.607 | 0.497 | |
| T stage | pT3 | pT4 | 1.619 | 0.678 | 3.869 | 0.278 | |
| **CF stroma ratio** | 0.167 | 0.271 | 0.469 | 0.245 | 0.895 | 0.062 | 0.616 |
| Differentiation | MD | PD | 1.233 | 0.485 | 3.131 | 0.66 | |
| Histological type | Adenocarcinoma | Mucinous | 0.51 | 0.119 | 2.188 | 0.364 | |
| T stage | pT3 | pT4 | 1.827 | 0.775 | 4.31 | 0.169 | |
| **CF necrosis ratio** | 0.022 | 0.052 | 0.619 | 0.302 | 1.267 | 0.202 | 0.552 |
| Differentiation | MD | PD | 1.504 | 0.577 | 3.919 | 0.404 | |
| Histological type | Adenocarcinoma | Mucinous | 0.695 | 0.16 | 3.018 | 0.627 | |
| T stage | pT3 | pT4 | 2.154 | 0.877 | 5.295 | 0.094 | |
| Appearance based tissue phenotypic features | | | | | | | |
| **AP smooth muscle ratio** | 0.143 | 0.34 | 2.086 | 1.025 | 4.247 | 0.127 | 0.563 |
| Differentiation | MD | PD | 1.359 | 0.507 | 3.641 | 0.542 | |
| Histological type | Adenocarcinoma | Mucinous | 0.437 | 0.1 | 1.913 | 0.272 | |
| T stage | pT3 | pT4 | 2.632 | 1.051 | 6.59 | **0.039*** | |
| **AP inflammation ratio** | 0.026 | 0.075 | 0.431 | 0.224 | 0.832 | **0.009*** | 0.625 |
| Differentiation | MD | PD | 0.938 | 0.347 | 2.535 | 0.9 | |
| Histological type | Adenocarcinoma | Mucinous | 0.822 | 0.185 | 3.642 | 0.796 | |
| T stage | pT3 | pT4 | 1.622 | 0.674 | 3.906 | 0.281 | |
| Other features | | | | | | | |
| **Morisita index (*Maley*)** | 0.34 | 0.533 | 0.742 | 0.397 | 1.387 | 0.646 | 0.502 |
| Differentiation | MD | PD | 1.254 | 0.481 | 3.272 | 0.643 | |
| Histological type | Adenocarcinoma | Mucinous | 0.551 | 0.128 | 2.375 | 0.424 | |
| T stage | pT3 | pT4 | 2.021 | 0.83 | 4.919 | 0.121 | |
| **Stroma-tumor ratio (*Mesker, West, Huijbers*)** | 0.37 | 0.594 | 0.813 | 0.464 | 1.424 | 0.583 | 0.515 |
| Differentiation | MD | PD | 1.167 | 0.436 | 3.124 | 0.759 | |
| Histological type | Adenocarcinoma | Mucinous | 0.617 | 0.14 | 2.714 | 0.523 | |
| T stage | pT3 | pT4 | 1.946 | 0.81 | 4.676 | 0.136 | |
| **Necrosis-tumor ratio (*Pollheimer, Richards, Jayasinghe*)** | 0.074 | 0.204 | 0.652 | 0.331 | 1.286 | 0.216 | 0.575 |
| Differentiation | MD | PD | 1.386 | 0.517 | 3.714 | 0.517 | |
| Histological type | Adenocarcinoma | Mucinous | 0.509 | 0.118 | 2.191 | 0.364 | |
| T stage | pT3 | pT4 | 1.873 | 0.784 | 4.474 | 0.158 | |
| **CF smooth muscle ratio** | 0.188 | 0.388 | 2.646 | 0.92 | 7.614 | **0.044*** | 0.608 |
| **AP inflammation ratio** | 0.037 | 0.102 | 0.705 | 0.291 | 1.707 | 0.19 | |
| Differentiation | MD | PD | 0.904 | 0.336 | 2.429 | 0.841 | |
| Histological type | Adenocarcinoma | Mucinous | 0.454 | 0.105 | 1.969 | 0.292 | |
| T stage | pT3 | pT4 | 2.575 | 1.015 | 6.535 | **0.047*** | |

* statistically significant result at the significance level 0.05
